# Supplementary material for: Surface Recombination Limited Lifetimes of Photoexcited Carriers in Few-Layer Transition Metal Dichalcogenide MoS2
Source: arXiv:1510.08563 source file (2015-11-02)
Supplement: Supplementary file 1 [file supp.pdf]

# Supplementary Information: Surface Recombination Limited Lifetimes of Photoexcited Carriers in Few-Layer Transition Metal Dichalcogenide $MoS_2$

Haining Wang,* Changjian Zhang, and Farhan Rana

*School of Electrical and Computer Engineering, Cornell University, Ithaca, NY, USA*

E-mail: hw343@cornell.edu

**Temperature Dependent Optical Conductivity Measurements in Multilayer $MoS_2$:** The real and imaginary parts,$\sigma_r$ and $\sigma_i$, respectively, of the optical conductivity of few-layer TMDs can be obtained by measuring their transmission and reflection spectra. Measured transmission and reflection spectra of few-layer $MoS_2$, with respect to the quartz substrate, are shown in Figure 1(a,b) for different layer numbers. The real part of the 2D optical conductivity $\sigma_r$ can be expressed in terms of these two measurements as follows,

$$\sigma_r(\omega) = \frac{(1+n_s)^2 - (1-n_s)^2 R(\omega)}{4\eta_o T(\omega)} - \frac{n_s}{\eta_o} \tag{1}$$

where $R(\omega)$ and $T(\omega)$ are the measured reflection and transmission spectra, respectively, with respect to the quartz substrate, $\eta_o$ is the vacuum impedance, and $n_s \approx 1.45$ is the substrate refractive index. Eq.(1) holds as long as the wavelengths of interest are much longer than the sample thickness. The imaginary part $\sigma_i$ can be obtained from either the transmission

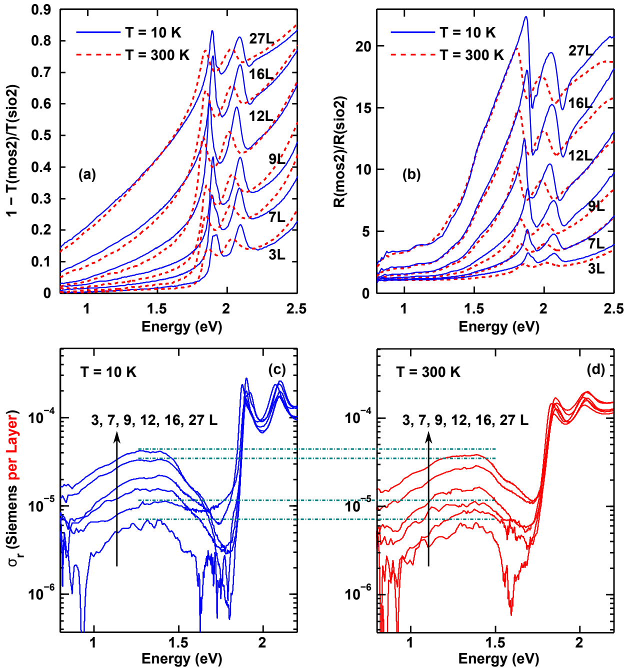


Figure 1: (a,b) Temperature dependent transmission and reflection measurements on few-layer $MoS_2$. (c,d) Real part of the optical conductivity of few-layer $MoS_2$, normalized to the number of layers, obtained from transmission and reflection measurements are plotted for two different temperatures, 10K and 300K.

or the reflection spectra once the real part $\sigma_r$ has been obtained, or, alternatively, it can be obtained from $\sigma_r$ by using Kramers-Kronig relations. $\sigma_r$ of few-layer $MoS_2$ with different number of layers, normalized to the number of layers, are plotted in Figure 1(c,d) for two different temperatures, 10K and 300K. Within the error margin of our measurements, $\sigma_r$ is seen to scale almost linearly with the number of layers. A weak absorption band was observed in all multilayer samples in the 0.8-1.6 eV range. Interestingly, this absorption band was not observed in monolayer samples.[1] We rule out indirect interband absorption as solely responsible for this absorption band since the band extends to energies much smaller than the indirect bandgap in even our thickest samples.[2,3] Since all our samples were n-doped, this absorption could be due to optical transitions from midgap defect states to the conduction bands or due to intraband optical transitions. Going from monolayer to multilayer TMD samples, the lowest conduction band and the highest valence band are expected to evolve into conduction and valence subbands, respectively,[2] in a manner similar to what happens

in semiconductor quantum wells, thereby allowing for intraband optical transitions. Note that $\sigma_r$ does not scale linearly with the number of layers in the 0.8-1.6 eV range.

Temperature dependent conductivity measurements were also performed and are also plotted in Figure 1 for two different temperatures, 10K and 300K. In the 0.8-1.6 eV absorption band, we find that $\sigma_r$ always increases with a decrease in the temperature. This observation seems consistent with the absorption band getting a strong contribution from midgap defect states whose occupation increases with a decrease in the temperature in our lightly n-doped samples.

**Details on the Carrier Recombination Dynamics:**

Defect-assisted electron and hole recombination in which carrier capture by defects occurs via Auger scattering is described by the following rate equations valid for our n-doped multilayer samples,[1,4]

$$\frac{dn}{dt} = -An_d n^2(1-F_d) \tag{2}$$

$$n_d\frac{F_d}{dt} = An_d n^2(1-F_d) - Bn_d npF_d \tag{3}$$

$$\frac{dp}{dt} = -Bn_d npF_d \tag{4}$$

Here, $n$ ($p$) is the electron (hole) density, $n_d$ is the defect density, $F_d$ is the defect occupation probability, and $A$ and $B$ are rate constants for Auger scattering. Electron and hole emission rates from the defects are ignored for simplicity.[1] It should be noted here that the photoexcited carrier dynamics in monolayer $MoS_2$ are not adequately described by the above set of equations.[1] In the case of monolayer $MoS_2$, fast defects contribute to rapid electron-hole recombination in the first few picoseconds, as observed experimentally.[1,5] The following discussion, therefore, holds only for multilayer samples. The equation for $F_d$ can be cast in the following form,

$$\frac{F_d}{dt} + (An^2 + Bnp)F_d = An^2 \tag{5}$$

Suppose we assume that $F_d$ evolves in time very fast and that it reaches a dynamic equilibrium value given by,

$$F_d \approx \frac{An}{An + Bp} \tag{6}$$

The condition for this fast evolution of $F_d$ is that the time scales over which it evolves are much shorter than the electron and hole capture times,

$$An^2 + Bnp >> An_d n(1 - F_d) \ , \ \ Bn_d p F_d \tag{7}$$

Our initial assumption would be self-consistently correct if,

$$An^2 + Bnp \quad >> \quad \frac{(Bn_d)(An_d)}{(An_d)n + (Bn_d)p} np \tag{8}$$

$$\Rightarrow An + Bp \quad >> \quad \frac{(Bn_d)(An_d)}{(An_d)n + (Bn_d)p} p \tag{9}$$

The above condition will generally hold if $n, p >> n_d$. In our experiments, the photoexcited carrier densities exceed $5 \times 10^{12}$ 1/cm$^2$ per layer or $8 \times 10^{19}$ 1/cm$^3$. We expect defect densities to be much smaller than these values. Using the dynamic equilibrium value of $F_d$, the rate equations for the electron and holes densities become,

$$\frac{dn}{dt} \approx \frac{dp}{dt} \approx -\frac{(An_d)(Bn_d)}{An_d n + Bn_d p} n^2 p \tag{10}$$

If the photoexcited electron and hole densities are much larger than the equilibrium electron density in our n-doped samples, which is the case in our experiments, then $n \approx p$, and the above Equation simplifies to the Equation given in the text,

$$\frac{dn}{dt} \approx \frac{dp}{dt} \approx -\frac{(An_d)(Bn_d)}{An_d + Bn_d} np \tag{11}$$

This material is available free of charge via the internet at http://pubs.acs.org.

# References

(1) Wang, H.; Zhang, C.; Rana, F. *Nano Letters* **2015**, *15*, 339–345, PMID: 25546602.

(2) Ellis, J. K.; Lucero, M. J.; Scuseria, G. E. *Applied Physics Letters* **2011**, *99*, –.

(3) Mak, K. F.; Lee, C.; Hone, J.; Shan, J.; Heinz, T. F. *Phys. Rev. Lett.* **2010**, *105*, 136805.

(4) Wang, H.; Strait, J. H.; Zhang, C.; Chan, W.; Manolatou, C.; Tiwari, S.; Rana, F. *Phys. Rev. B* **2015**, *91*, 165411.

(5) Docherty, C. J.; Parkinson, P.; Joyce, H. J.; Chiu, M.-H.; Chen, C.-H.; Lee, M.-Y.; Li, L.-J.; Herz, L. M.; Johnston, M. B. *ACS Nano* **2014**, *8*, 11147–11153, PMID: 25347405.
